# Supplementary material for: Pseudo-Labeling for Domain-Agnostic Bangla Automatic Speech Recognition
Source: arXiv:2311.03196 source file (2023-11-06)
Supplement: Supplementary file 1 [file appendix.tex]

\section{More details on Psedu-annotation}
\label{sec:details_psedu_annotation}

The MegaBNCorpus offers a significant contribution to the field of Bangla ASR research Its large-scale nature, comprising 18,000 hours of training data, provides a substantial resource for training state-of-the-art ASR models. Additionally, the provided test sets can be used for evaluating and benchmarking new models. 

Our pseudo-labeling annotation strategy provides an important direction to be dependent on machine-generated labeling in case of large unlabeled datasets.

% \begin{table*}
% \centering
% \begin{tabular}{ll}
% \hline
% \textbf{Human Annotation} & \textbf{Psedu Annotation}   \\
% \hline
% ফের সিবিআই তলব ভোট পরবর্তী অশান্তি মামলায় অনুব্রত কে তলব করে সিবিআই আজ & \ফের সিবিআই তলব ভোট পরবর্তী অশান্তি মামলায় অনুব্রত কে তলব করে সিবিআই \\
% % মানুষ ঠিকই বাড়িতে যাচ্ছে কিন্তু অনেক কষ্টের মাধ্যমে ঈদের পূর্বের একটা শুক্রবার সে কারণে আজকের & মানুষ ঠিকই বাড়িতে যাচ্ছে কিন্তু অনেক কষ্টের মাধ্যমে এদের পূর্বের একটা শুক্রবার সে কারণে আজকের  \\

% % নাই যেটা আমরা আগে দেখেছি সো আমার মনে হয় এখন এই & নাই যেটা আমরা আগে দেখেছি আমার মনে হয় এখন এই  \\
% \hline
% \end{tabular}
% \caption{\label{category_wise_test_set_evaluation}
% A set of examples of Psedu annotation and human annotation
% }
% \end{table*}

\begin{figure}
    \centering
    \includegraphics[width=0.47\textwidth]{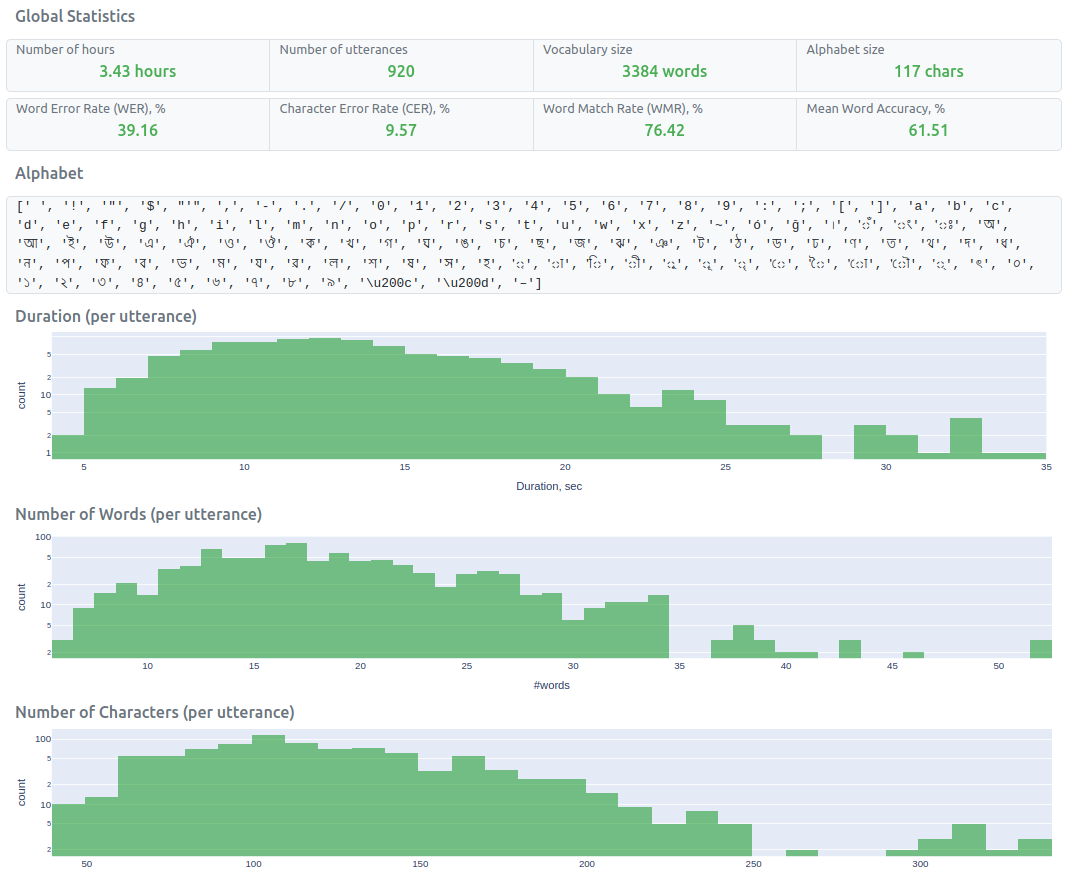}
    \caption{Nemo Data Visualization for hishab baseline model transcription on fleurs testset
    }
    \label{fig:fluers_hishab}
\end{figure}

\begin{figure}
    \centering
    \includegraphics[width=0.47\textwidth]{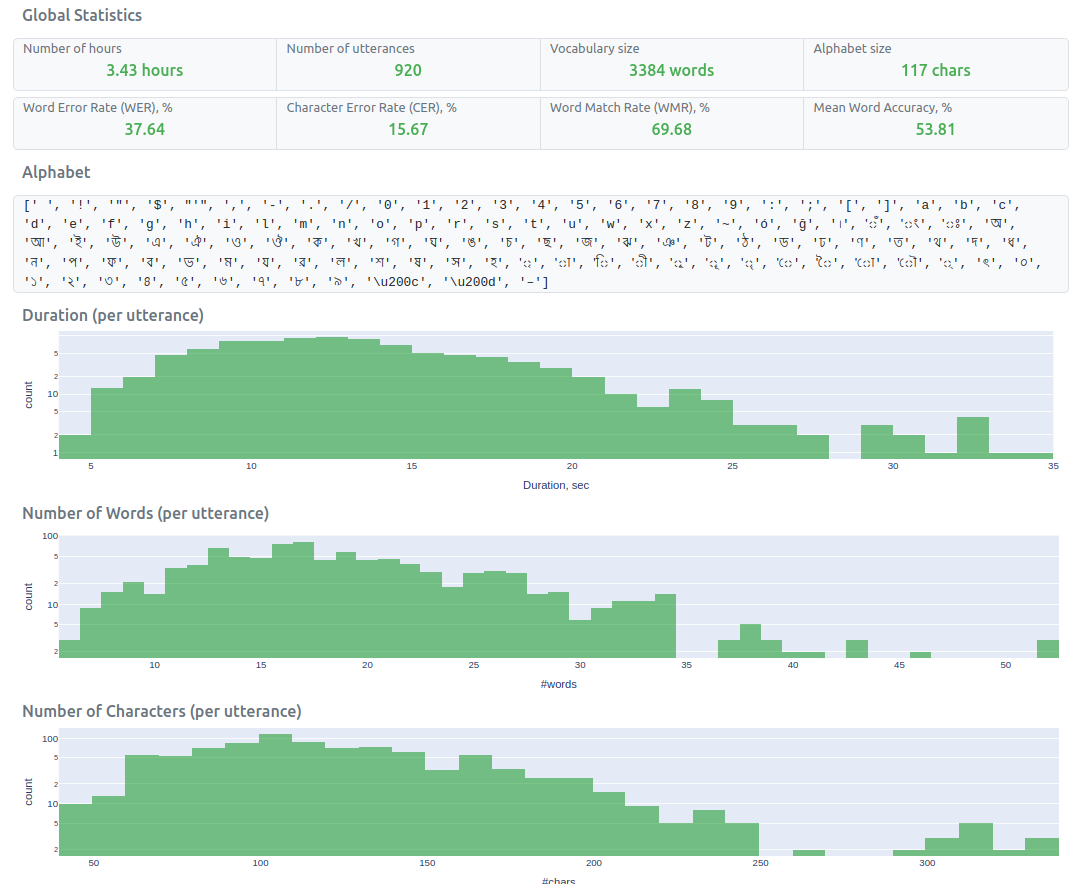}
    \caption{Nemo Data Visualization for BengaliAI Conformer model transcription on fleurs testset
    }
    \label{fig:fleurs_bengaliASR}
\end{figure}
